# Supplementary material for: Enhancing Online Road Network Perception and Reasoning with Standard Definition Maps
Source: arXiv:2408.01471 source file (2024-08-01)
Supplement: Supplementary file 1 [file X_suppl.tex]

\clearpage
\setcounter{page}{1}
\maketitlesupplementary
\appendix

\begin{figure*}[t]
  \centering
   \includegraphics[width=.9\textwidth]{figures/appendix/perception_additional_challenging_cases_2.pdf}
   \caption{Visualization for challenging cases in online perception task. Occlusion becomes a challenge when many vehicles are on a narrow street with tall buildings. SD maps provide valuable prior in these cases.}
   \label{fig:sup-perception-vis-1}
\end{figure*}

\section{Metrics} \label{sec:sup-metrics}
\textbf{Perception-only Metrics}
For the perception-only task, we evaluate the proposed architecture using Chamfer distance~\cite{liu2023vectormapnet, MapTR}, Fréchet distance~\cite{gao2020vectornet, wang2023openlanev2}, and Fréchet distance with permutation.

Chamfer distance characterizes the distance of two point sets $\{\mathcal{S}_1, \mathcal{S}_2\}$, in this case prediction and groundtruth pair $\{D_L^k, GT_L^m\}$. The Directional Chamfer distance is given by
\begin{equation}
    \text{CD}_{\text{dir}}(\mathcal{S}_1, \mathcal{S}_2) =  \frac{1}{|\mathcal{S}_1|} \sum_{p \in \mathcal{S}_1} \min_{q \in \mathcal{S}_2} ||p - q||_2.
\end{equation}
The norm is the Euclidean distance between points. Directional Chamfer distance is asymmetrical hence bidirectional Chamfer distance is used here, defined by 
\begin{equation}
    \text{CD}(\mathcal{S}_1, \mathcal{S}_2) = \frac{1}{2} \left ( \text{CD}_{\text{dir}}(\mathcal{S}_1, \mathcal{S}_2) + \text{CD}_{\text{dir}}(\mathcal{S}_2, \mathcal{S}_1) \right ). 
\end{equation}

% \begin{equation}
%     \text{CD}(D_L^k, GT_L^m) = \frac{1}{2} \left ( \frac{1}{N_L} \sum_{j=1}^{N_{L}} \min_{x_n^m \in GT_L^m} (\mathbf{x}_j^k - \mathbf{x}_n^m)^2 + \frac{1}{N_L} \sum_{n=1}^{N_{L}} \min_{\mathbf{x}_j^k \in D_L^k} (\mathbf{x}_j^k - \mathbf{x}_n^m)^2 \right ). 
% \end{equation}

% \red{Need formal definition, see reference in TopoNet, VectorMapNet, OpenLane-V2}

Chamfer distance only captures the point sets distance but misses the order. Fréchet distance takes the order into account. It measures the distance between two curves. In the case of the curve being discrete, we use Discrete Fréchet Distance instead. Given two curves $\mathcal{S}_1 = \{p_1, p_2, \cdots, p_n\}$ and $\mathcal{S}_2 = \{q_1, q_2, \cdots, q_m\}$, a coupling $C$ is a list of index pairs defined as $C = \{(a_1, b_1), (a_2, b_2), \cdots, (a_k, b_k)\}$ such that the indexes satisfy the start point and end point condition $a_1 = b_1 = 1$, $a_k = n$, $b_k = m$, but also incrementally and monotonically traverse the two curves $a_{i+1} = a_{i}$ or $a_{i+1} = a_{i} + 1$ and $b_{i+1} = b_{i}$ or $b_{i+1} = b_{i} + 1$. For a specific coupling $C$, the distance $D_C$ is defined as 
\begin{equation}
    D_C = \max_{i = 1}^k || a_i - b_i ||_2, 
\end{equation}
the maximum distance between any pair of points in the coupling. The Discrete Fréchet Distance FD is defined as 
\begin{equation}
    \text{FD}(\mathcal{S}_1, \mathcal{S}_2) = \min_{\forall C} D_C,
\end{equation}
 the minimum distance of the two curves for all couplings and can be solved by dynamic programming in polynomial time. %~\cite{eiter1994frechetdistance}.

While Fréchet distance captures the direction, it also weighted significantly on the direction. For example, if we define $\Bar{\mathcal{S}}_2 = \{ q_m, q_{m-1}, \cdots, q_1 \}$, which is the curve $\mathcal{S}_2$ reversing order, . The Frechet distance of FD$(\mathcal{S}_1, \Bar{\mathcal{S}}_2)$ can change drastically from FD$(\mathcal{S}_1, \mathcal{S}_2)$. Can we both capture the order but penalize less on the direction? That motivates us to use Fréchet distance with permutation FD$_p$. Thus we have 
\begin{equation}
    \text{FD}_p (\mathcal{S}_1, \mathcal{S}_2) = \min \left (\text{FD} (\mathcal{S}_1, \mathcal{S}_2), \text{FD} (\mathcal{S}_1, \Bar{\mathcal{S}}_2) \right ).
\end{equation}
In the case of centerline estimation, we calculate the Fréchet distance of the prediction against groundtruth in both directions and take the minimum.
% \section{Rationale}
% \label{sec:rationale}
% % 
% Having the supplementary compiled together with the main paper means that:
% % 
% \begin{itemize}
% \item The supplementary can back-reference sections of the main paper, for example, we can refer to \cref{sec:intro};
% \item The main paper can forward reference sub-sections within the supplementary explicitly (e.g. referring to a particular experiment); 
% \item When submitted to arXiv, the supplementary will already included at the end of the paper.
% \end{itemize}
% % 
% To split the supplementary pages from the main paper, you can use \href{https://support.apple.com/en-ca/guide/preview/prvw11793/mac#:~:text=Delete%20a%20page%20from%20a,or%20choose%20Edit%20%3E%20Delete).}{Preview (on macOS)}, \href{https://www.adobe.com/acrobat/how-to/delete-pages-from-pdf.html#:~:text=Choose%20%E2%80%9CTools%E2%80%9D%20%3E%20%E2%80%9COrganize,or%20pages%20from%20the%20file.}{Adobe Acrobat} (on all OSs), as well as \href{https://superuser.com/questions/517986/is-it-possible-to-delete-some-pages-of-a-pdf-document}{command line tools}.

\textbf{Perception and Reasoning Metrics}
The TopoNet~\cite{li2023toponet} and OpenLane-V2~\cite{wang2023openlanev2} introduced a new set of metrics to encompass perception and reasoning capabilities. 

The perception metrics are composed of a centerline detection component (DET$_l$) and a traffic element detection component (DET$_t$). Using Fréchet distance as earlier described, DET$_l$ corresponds to the mean average precision of centerline detection over three association thresholds $\{1.0, 2.0, 3.0\}$. Additionally, a relaxation factor is added to the Fréchet distance calculation in the OpenLane-V2 evaluation for far-range objects. The final results are averaged across all three thresholds as shown below, where $A P_t$ denotes the average precision associated with threshold $t$.

\begin{equation}
\mathrm{DET}_l=\frac{1}{|\mathbb{T}|} \sum_{t \in \mathbb{T}} A P_t
\end{equation}

Additionally, DET$_t$ is calculated based on Intersection over Union (IoU) for a specific traffic element class $e$ and then averaged across all traffic element classes ($\mathbb{E}$).

\begin{equation}
    \mathrm{DET}_t=\frac{1}{|\mathbb{E}|} \sum_{e \in \mathbb{E}} A P_e
\end{equation}

The OpenLane-V2 benchmark additionally introduces reasoning metrics for topology estimation, TOP$_{ll}$ and TOP$_{lt}$. These metrics are in particularly relevant for evaluating the relational attributes among centerlines and between centerlines and traffic elements.
The evaluation of graph predictions applies to both metrics. 

Given a ground truth graph $G=(V, E)$ and a prediction $\hat{G}=(\hat{V}, \hat{E})$, a projection is first created as denoted by $G'=(V', E')$ that enforces a number of requirements, $V = \hat{V}'$, $\hat{V}' \subseteq \hat{V} \cup V_d$, where $V_d$ is a set of placeholders (i.e dymmy vertices). In this context, Fréchet and IoU are reused to calculate true positives of centerlines and traffic elements, respectively. Given that the graph connectivity is of relevance for the task, a connection is inferred if the confidence associated with an edge predicted from the adjacency matrix is greater than a fixed threshold ($0.5$). For a given vertex $v$, the corresponding neighbors are then calculated by $\mathcal{N}(v)$ and the precision associated with the vertex (centerline or traffic element ) is given by $\mathcal{P}(v)$. The overall metric utilized is then characterized as follows, where $\mathbbm{1}(\cdot)$ is an indicator function. 

\begin{equation}
    \mathrm{TOP}=\frac{1}{|V|} \sum_{v \in V} \frac{\sum_{\hat{n}^{\prime} \in \hat{\mathcal{N}}^{\prime}(v)} \mathcal{P}\left(\hat{n}^{\prime}\right) \mathbbm{1}\left(\hat{n}^{\prime} \in \mathcal{N}(v)\right)}{|\mathcal{N}(v)|}
\end{equation}

\section{Perception Task} \label{sec:sup-perception}

\subsection{Losses in Perception task} \label{sec:sup-loss-perception}

The losses are the same as introduced in~\cite{MapTR}, a correspondence is established by matching the prediction and groundtruth with minimum point-to-point distance, then the total loss is a weighted sum of classification loss $\mathcal{L}_{cls}$, point distance loss $\mathcal{L}_{p2p}$ and edge directional loss $\mathcal{L}_{dir}$ given by

\begin{equation}
    \mathcal{L} = \lambda \mathcal{L}_{cls} + \alpha \mathcal{L}_{p2p} + \beta \mathcal{L}_{dir}.
\end{equation}

The classification loss $\mathcal{L}_{cls}$ is the Focal Loss of the predicted class $\hat{c}_i$ and matched groundtruth class $c_i$.
\begin{equation}
    \mathcal{L}_{cls} = \sum_{i=0}^{N_m-1} \mathcal{L}_{\text{Focal}}(\hat{c}_i, c_i).
\end{equation}

The map elements geometry are supervised by both the point-to-point loss $\mathcal{L}_{p2p}$ and edge-to-edge loss $\mathcal{L}_{dir}$. The point-to-point loss reduces the local error of each corresponding point in matched pairs of prediction and groudtruth, given by 

\begin{equation}
    \mathcal{L}_{p2p} = \sum_{i=0}^{N_m-1} \mathbbm{1}_{c_i \neq \varnothing} \sum_{j=0}^{N_L-1} D_{Manhattan}(\hat{\mathbf{v}}_j, \mathbf{v}_j), 
\end{equation}

where the $\hat{\mathbf{v}}_j$ is the matched point in prediction to groundtruth point $\mathbf{v}_j$ that minimize the total point-to-point distance. 

The edge-to-edge loss $\mathcal{L}_{dir}$ constraints the direction of the matched edges to be similar which adds additional relational information to the loss.

\begin{equation}
    \mathcal{L}_{dir} = \sum_{i=0}^{N_m-1} \mathbbm{1}_{c_i \neq \varnothing} \sum_{j=0}^{N_L-1} \textit{cosine\_similarity}(\hat{\mathbf{e}}_j, \mathbf{e}_j). 
\end{equation}

\begin{figure*}[t]
  \centering
   \includegraphics[width=.9\textwidth]{figures/appendix/perception_map_inconsistency_cases_2.pdf}
   \caption{Visualization for map inconsistency in perception task. Groundtruth and OpenLane-V2 SD maps may not agree with each other leading to confusion.}
   \label{fig:sup-perception-vis-2}
\end{figure*}

\subsection{Qualitative Results} \label{sec:sup-perception-qualitative-results}

We provide more qualitative results from the evaluation set of OpenLane-V2 to understand why the SD maps improve the performance significantly. As shown in~\cref{fig:sup-perception-vis-1}, in the challenging scenes where there are heavy occlusion, due to many vehicles, trees, buildings and narrow streets, the baseline struggles while our model leveraging SD map prior maintains better road structure.

There are also many cases where our method struggles, as shown in~\cref{fig:sup-perception-vis-2}. For example, the inconsistencies between OpenLane-V2 SD maps and groundtruth maps can lead to confusion in training. Thus in evaluation there are some cases the model cannot predict the road structure with a confidence above certain threshold (in these visualizations 0.4 is used).

More qualitative results similar to~\cref{fig:perception-sdmap} are located in \textit{supplementary-videos/figure6/}.

% \newpage

\section{Perception and Reasoning Task}
\subsection{Scene Graph Neural Network Components}
\label{sup:sgnn}

The first SGNN component leverages the centerline-centerline graph from the previous layer $G^{i-1}_{CC}$ to update the centerline queries generated by the Centerline Deformable Decoder and the Multi-Head Attention mechanism blocks. It additionally embeds directional information of centerlines in the feature propagation formulation by introducing a learnable weight matrix $\mathbf{W}_{CC}^i$. By noting that $Q^i_{C} = \left\{Q^i_{C(m)}\right\}_{m=1}^{M_l}$, a corresponding centerline query $C(m)$ can be updated by the following propagation process in the first SGNN component.

% --------------------
\begin{equation}
\begin{aligned}
\label{eq3.2.5}
Q_{C(m)}^{i(1)}=\sum_{\forall n \in \mathcal{N}(m)} \sum_{\forall c_l \in C_l} \alpha T_{CC\left(c_l, m, n\right)}^{i-1} \mathbf{W}_{CC\left(c_l\right)}^i Q_{C(n)}^i \\
T_{CC\left(c_l, m, n\right)}^{i-1}=\operatorname{stack}\left(A_{CC}^{i-1}, \left(A_{CC}^{i-1}\right)^\top, I\right)
\end{aligned}
\end{equation}

% --------------------
~\cref{eq3.2.5} leverages a learnable weight between centerlines, $\mathbf{W}_{CC}^i \in \mathbb{R}^{\left|C_l\right| \times F_c \times F_c}$ and a secondary weight matrix defined by $T_{CC}^{i-1}\in \mathbb{R}^{\left|C_l\right| \times F_c \times F_c}$ to control the flow of messages and enable bidirectional message exchange between two connected centerlines and self-loops. In other words, $T_{CC}^{i-1}$ leverages $A^i_{CC}$ to encode three different connection modes: $\{successor, predecessor, self\text{-}loop\}$.

\begin{equation}
\begin{aligned}
\label{eq3.2.6}
Q_{C{(m)}}^{i(2)}=\sum_{\forall n \in \mathcal{N}(m)} \sum_{\forall c_l \in C_l} \mathbf{X} \cdot \mathbf{W}_{CT\left(c_l\right)}^i \cdot f^{(i)}_{proj}\left(Q_{T(n)}^i\right), \\
\mathbf{X} = \beta S_{T\left(c_l, n\right)}^i A_{CT(m,n)}^i
\end{aligned}
\end{equation}

The second SGNN component integrates traffic element queries and centerline queries as shown in~\cref{eq3.2.6}. Similar to~\cref{eq3.2.5}, $\mathbf{W}_{CT} \in \mathbb{R}^{\left|C_l\right| \times F_c \times F_t}$ is a learnable weight matrix; however, the traffic sign classification scores $S_T^i \in \mathbb{R}^{\left|C_t\right| \times \left|Q^i_T\right|}$ are additionally used as a weight, where $\left|C_l\right|$ corresponds to the number of traffic element classes, $\left|Q^i_T\right|$ the number of queries, $F_c,F_t$ correspond to the feature embedding dimension of a centerline query, and a traffic element, respectively. Since the traffic elements are predicted in a image reference view, an additional embedding network $f^{(i)}_{proj}$ is used to extract semantic features from the traffic element queries and unify them in BEV space. A different embedding network is indexed by $i$ for each of the decoder layers. $\alpha , \beta$ denote hyperparameters.

\subsection{Losses in Perception and Reasoning Task}
\label{sup:perception-reasoning-loss}
The detection loss components for traffic elements and centerlines ($\mathcal{L}_{T}$ and $\mathcal{L}_{C}$) leverage a Bipartite Matching loss introduced in DETR~\cite{carion2020detr} to match predictions to ground truth labels, where the traffic elements predicted by the perception heads are generated using $Q^i_T$ and the centerline elements are predicted using queries $Q^i_C$
\label{perception-reasoning-losses}. The traffic element perception head generates 2D bounding box coordinates as well as confidence scores for each class while the centerline head generates 11 3D keypoints for each centerline. After the matching process, $\mathcal{L}_{T}$ is calculated using an IOU loss, an L1 loss for bounding box regression and the Focal loss~\cite{lin2017focal} for classification. On the other hand, the centerline perception loss $\mathcal{L}_{C}$ is a combination of the Focal loss and L1 loss.

To determine the relational information among centerlines and between centerlines and traffic elements, an MLP is utilized to condense the feature dimensions in combination with a sigmoid activation function to score their relationship. The Focal loss ($\mathcal{L}_{rel}$) is then utilized for the reasoning component task. An important note to make in the use of traffic element embeddings to measure their association with centerlines is that the embedding network $f^{(i)}_{proj}$ from~\cref{eq3.2.6} is used to ensure that relational features that are represented in an unified perspective, namely BEV since the traffic element embeddings are initially extracted from a perspetive view. The total loss for reasoning is then $\mathcal{L}=\mathcal{L}_{T}+\mathcal{L}_{C} + \mathcal{L}_{rel}$.

% \clearpage
% \newpage
\subsection{Qualitative Results}
\label{sup:perception-reasoning-visuals}
Additional qualitative comparisons between the TopoNet baseline (Toponet-R50) and our method can be found in~\cref{sup:perception-reasoning-vis-1}. This comparison show cases a number of scenarios with light to severe occlusion from static and dynamic objects, clearly highlighting the benefits of our proposed method (TopoOSMR). Complete scenario videos are located under \textit{supplementary-videos/figure1/} and \textit{supplementary-videos/figure9/}. 

\begin{figure*}[t]
  % \vspace{0.2cm}
  \centering
   \includegraphics[width=.9\textwidth]{figures/appendix/toposmr_sup_appendix.pdf}
   \caption{Online road network perception and reasoning visualizations corresponding to Toponet-R50 (baseline) and our method (TopoOSMR) which leverages rasterized SD maps. Visualizations represent centerlines with connectivity information corresponding to four test cases (rows) from OpenLane-V2 dataset.}
   \label{sup:perception-reasoning-vis-1}
\end{figure*}

% \begin{figure*}[h]
%   % \vspace{0.2cm}
%   \centering
%    \includegraphics[width=.9\textwidth]{figures/appendix/toposmr_sup_2.pdf}
%    \caption{TODO.}
%    \label{sup:perception-reasoning-vis-2}
% \end{figure*}

% \begin{figure*}[h]
%   % \vspace{0.2cm}
%   \centering
%    \includegraphics[width=.9\textwidth]{figures/appendix/toposmr_sup_3.pdf}
%    \caption{TODO.}
%    \label{sup:perception-reasoning-vis-3}
% \end{figure*}

% \clearpage
% \newpage

\section{OpenLane-V2-OSM Details}
\label{sup:dataset-osm}
% \subsection{OpenLane-V2-OSM Details}
The OpenStreetMaps (OSM) files generated are used as enhancements for the existing OpenLane-V2 dataset (subset-A) that is based on the Argoverse 2 dataset. In total, there are 1,000 dataset scenarios divided into 750 training, 150 validation, and 150 testing. For each scenario, we analyze the ego-vehicle poses to extracted the bounded region that covers the ego-vehicle poses with an added minimum of 200m lateral and longitudinal  horizon. This bounded region is then used to fetch the maps using the OSM API and adapt the XML and PBF data formats to preserve map original map information while providing  a convenient  processing format; both files are lightweight. The map data is further processed into a PKL data format using NetworkX %~\cite{SciPyProceedings_11}
to facilitate data loader implementations and training processes. This process aligns each of the OpenLane-V2 data segments with an ego-centric OSM map (in raster and graph versions) by utilizing the available localization traces. A projection is performed to convert a WGS84 format into cartesian space. Lastly, we incorporate a number of node attributes by leveraging the OSM nodes and edges. In the experiments outlined in~\cref{sec:perception-reasoning-results}, we extract 25 attributes corresponding to the \textit{highway} way category (edge type): 
% $\{ crossing, living\_street, mini\_roundabout, motorway,$
% $motorway\_junction, motorway\_link, path,$ 
% $primary\_link, residential, road, secondary,$ $secondary\_link, service, services, stop, tertiary,$ $tertiary\_link, traffic\_sign, traffic \_signals,$ $trunk, trunk\_link, turning\_circle, turning\_loop,$ $unclassified\}$. 

\begin{table}[h]
\centering
\resizebox{\columnwidth}{!}{%
\begin{tabular}{ccccc}
crossing       & living\_street & mini\_roundabout & motorway      & motorway\_junction \\
motorway\_link & path           & primary          & primary\_link & residential        \\
road           & secondary      & secondary\_link  & service       & services           \\
stop           & tertiary       & tertiary\_link   & traffic\_sign & traffic\_signals   \\
trunk          & trunk\_link    & turning\_circle  & turning\_loop & unclassified      
\end{tabular}%
}
\caption{OSM \textit{highway} way attributes utilized to extract road elements in rasterized and graph based representations. The road include small to large urban driving road classes, as well as turning circles.}
\label{sup:osm-classes}
\end{table}

Note: during the data loading process in training, the OSM maps are interpolated to ensure that node attributes are equal-distant to one another. In the experiments described in this work, we utilize a $1m/waypoint$ density factor.

\section{Limitations}
\label{sup:dataset-limitations}
% \subsection{Data Diversity}
% \label{sup:dataset-diversity}
Argoverse2/OpenLane-V2 includes diverse road topologies that may be out of the distribution of the training set as shown in~\cref{sup:data-diversity}. Complete scenario videos are located under \textit{supplementary-videos/figure10/}.

\begin{figure*}[H]
  % \vspace{0.2cm}
  \centering
   \includegraphics[width=.9\textwidth]{figures/appendix/toposmr_sup_5.pdf}
   \caption{Online road network perception and reasoning visualizations corresponding to Toponet-R50 (baseline) and out method (TopoOSMR) which leverages rasterized SD maps. The test sample from OpenLane-V2 showcases a complex five-way urban intersection.}
   \label{sup:data-diversity}
\end{figure*}

\subsection{Duplicates}
\label{sup:dataset-duplicates}
While the datasets utilized in our experiments are diverse, data segments often include overlapping geographic data as shown in~\cref{sup:data-duplicates}. This may indicates a potential need for data augmentation and model generalizability.  

\begin{figure*}[H]
  % \vspace{0.2cm}
  \centering
   \includegraphics[width=.9\textwidth]{figures/appendix/dataset-duplicates.pdf}
   \caption{Two dataset scenarios from the OpenLane-V2 dataset are shown (top and bottom row). Although the data corresponds to two different data samples, the overlapping data corresponds to the same geographic location. Groundtruth road networks shown on the left.}
   \label{sup:data-duplicates}
\end{figure*}

\subsection{Label Consistency}
\label{sup:dataset-consistency}
We observe scenarios where the ground truth labels deviate from perception data. In~\cref{sup:limitations-consistency}, we observe centerline definitions that may lead to a traffic rule violation if double solid lines are crossed. This highlights an important aspect of future work which entails map consistency and traffic rules. Complete scenario videos are located under \textit{supplementary-videos/figure12/}.

\begin{figure*}[H]
  % \vspace{0.2cm}
  \centering
   \includegraphics[width=.9\textwidth]{figures/appendix/toposmr_sup_4.pdf}
   \caption{Ground truth centerline definitions and connections (left) lead to a solid lane cross which may indicate traffic rule violation.}
   \label{sup:limitations-consistency}
\end{figure*}
